# Supplementary material for: Contactless estimation of continuum displacement and mechanical compressibility from image series using a deep learning based framework
Source: arXiv:2602.07065 source file (2026-02-05)
Supplement: Supplementary file 1 [file Supplementary_information.pdf]

# Supplementary Information

A.N.Maria Antony, T. Richer, E. Gladilin

Contactless determination of continuum displacement and mechanical compressibility from image series using a deep learning based framework

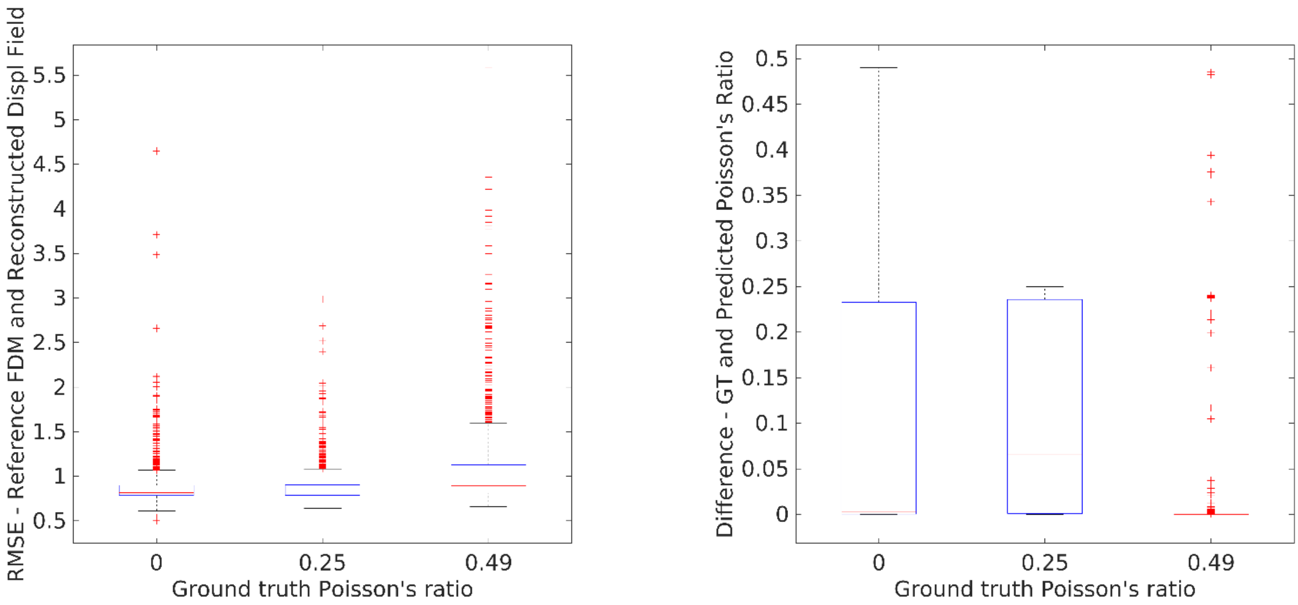


**Figure S1**: (Left) RMSE of the error between reference FDM and displacement fields reconstructed from image registration in dependence on the Poisson's ratio. (Right) Difference between ground truth and predicted Poisson's ratio using the DNN model trained with pure FDM and validated against displacements reconstructed from image registration as a function of ground truth Poisson's ratio.

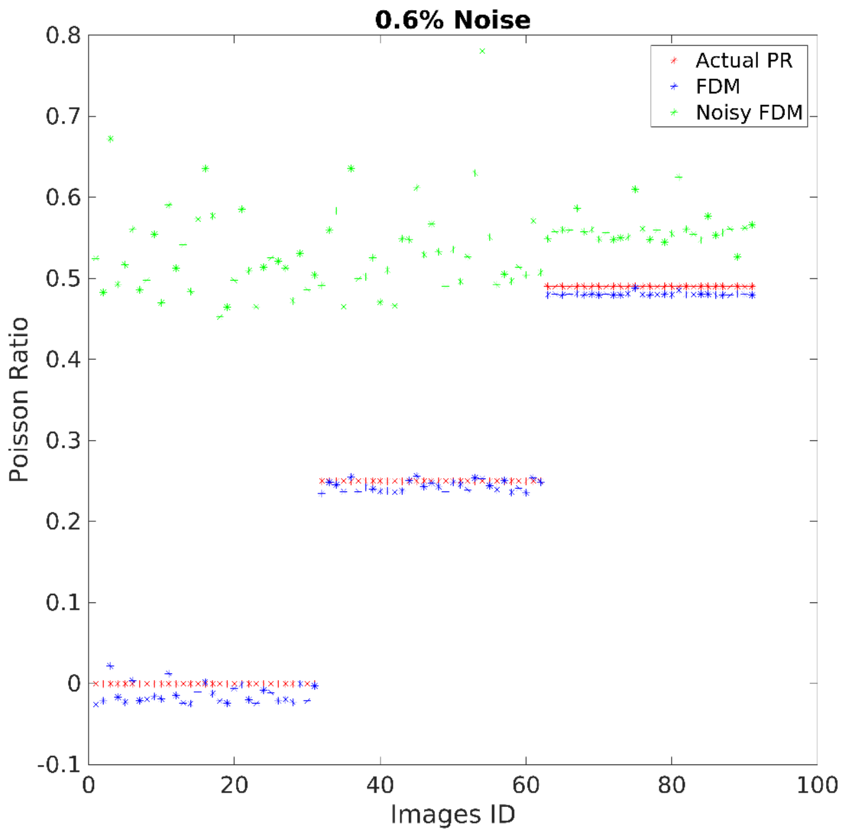


**Figure S2**: Estimation of the Poisson's ratio from original (blue) vs. noisy (green) image displacement using analytic equation (Eq. 7, main text). Red labels indicate true values of the Poisson's ratio. Already a moderate level of 0.6% additive noise leads to sever errors in estimation of material's compressibility, because it is very sensitive to relative proportion of XY displacement components.

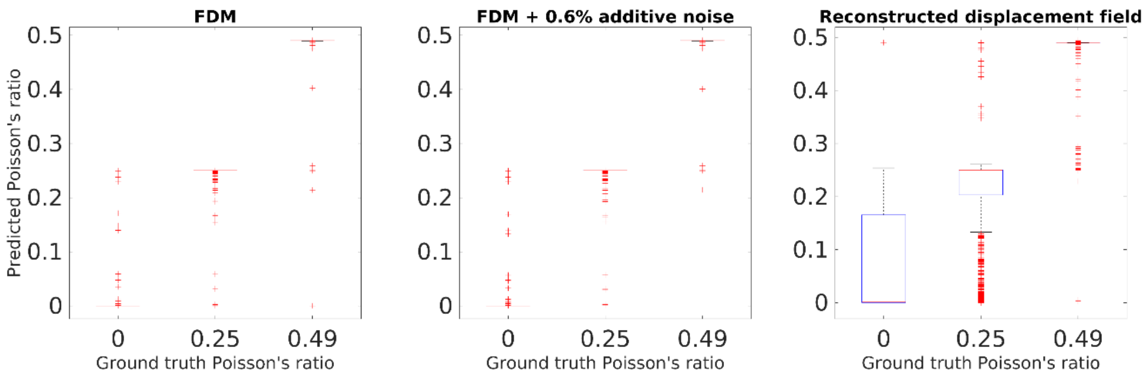


**Figure S3**: Boxplot visualization of the Poisson's ratio distributions obtained for all test images re. displacement fields using DNN model trained using FDM + 5% Noise: (left) displacement obtained as an exact FDM solution, (middle) FDM-computed displacement overlaid with 0.6% additive noise and (right) displacement fields reconstructed from image registration.

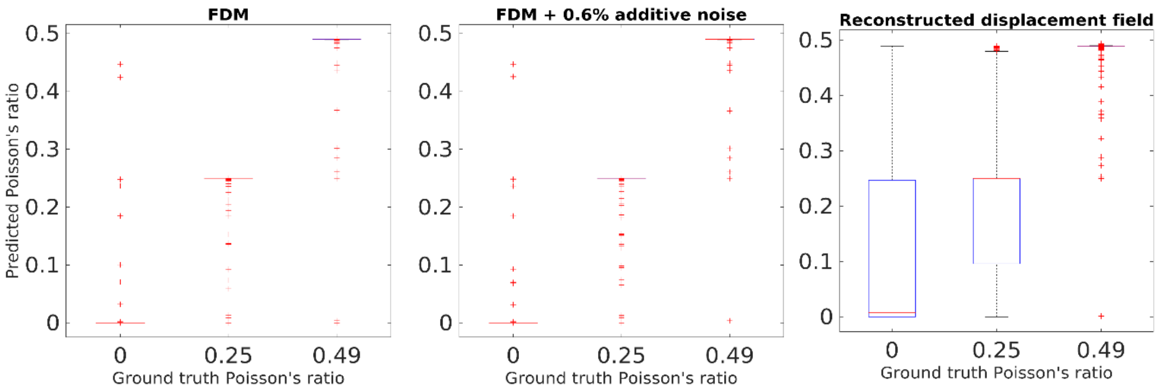


**Figure S4**: Boxplot visualization of the Poisson's ratio distributions obtained for all test images re. displacement fields using DNN model trained using FDM + 10% Noise: (left) displacement obtained as an exact FDM solution, (middle) FDM-computed displacement overlaid with 0.6% additive noise and (right) displacement fields reconstructed from image registration.
